# Supplementary material for: Turbulent mixing controls fixation of growing antagonistic populations
Source: arXiv:2408.16784 ancillary file (2024-08-22)
Supplement: Supplementary file 1 [file SI.pdf]

# Supplementary Information for

## Turbulent mixing controls fixation of growing antagonistic populations

**Jonathan Bauermann, Roberto Benzi, David R. Nelson, Suraj Shankar and Federico Toschi**

**Corresponding Author name.**
**E-mail: drnelson@fas.harvard.edu**

### This PDF file includes:

Supplementary text
Figs. S1 to S2
Table S1
Legend for Movie S1
SI References

### Other supplementary materials for this manuscript include the following:

Movie S1

## Supporting Information Text

Here, we provide supporting information and arguments about the results obtained in the main text. In the first section, we explain how the velocity field can be rescaled to obtain different Damköhler numbers in the numerical simulations. In the second section, we explain how the critical fraction for fixation was determined. In the third section, we check the influence of different initial shapes on the critical fraction needed for fixation, and in the fifth section, we show the difference in total concentration fluctuations in antagonistic genetic mixtures compared to a passive scalar.

## 1. Scaling properties on the advected fields under turbulent flow

For obtaining numerical results for different Damkhler numbers Da=$\mu L/v_{\rm rms}$, we reused the same velocity fields but rescaled their magnitude. Therefore, we kept $\mu$ and $L$ constant but rescaled $v_{\rm rms}$ in the dynamics of $c_A$ and $c_B$, and altered the time scale correspondingly. This practice has many advantages from a computational point of view. First, we do not need to change the grid resolution upon changing $\mu$. Second, we can use the same turbulent flow fields for many different settings of Damköhler numbers (as long as we are in the limit that the dynamics of the concentrations $c_A$ and $c_B$ do not couple back to the dynamics of the velocity $\mathbf{v}$), without solving the computationally expensive Navier-Stockes equations, but rather solving it once and storing the velocity fields. Third, we can directly compare concentration fields with different Damköhler numbers but the same rescaled flow fields, as done, for example, in Fig. 1.

Here, we explain in detail the performed scaling. Let us start by restating the equation of motion we consider:

$$\partial_t f + \lambda \mathbf{v}\cdot\nabla f = D\nabla^2 f + \mu f(1-f)\left[\frac{\delta}{2} + \sigma(2f-1)\right] \quad \text{[S1]}$$

$$\partial_t \mathbf{v} + \mathbf{v}\cdot\nabla\mathbf{v} = -\frac{1}{\rho}\nabla p + \nu\nabla^2\mathbf{v} \quad \text{[S2]}$$

where $\lambda$ is a dimensionless free scaling parameter. We want to understand what the physical meaning of changing $\lambda$ corresponds to. For this purpose, we consider the transformation

$$t = \frac{1}{\lambda}\tilde{t}, \quad \text{[S3]}$$

$$D = \lambda\tilde{D}, \quad \text{[S4]}$$

$$\mu = \lambda\tilde{\mu}. \quad \text{[S5]}$$

With the transformation above, Eq. (S1) becomes

$$\partial_{\tilde{t}} f + \mathbf{v}\cdot\nabla f = \tilde{D}\nabla^2 f + \tilde{\mu} f(1-f)\left[\frac{\delta}{2} + \sigma(2f-1)\right]. \quad \text{[S6]}$$

Note that under this transformation, the interface width (Fisher scale) $w = 2\sqrt{D/(\mu\sigma)}$ is left invariant.

Next we observe that the Navier-Stokes Eq. (S2) is invariant under the transformation:

$$t = \frac{1}{\lambda}\tilde{t}, \quad \text{[S7]}$$

$$\mathbf{v} = \lambda\tilde{\mathbf{v}}, \quad \text{[S8]}$$

$$\nu = \lambda\tilde{\nu}, \quad \text{[S9]}$$

$$p = \lambda^2\tilde{p}. \quad \text{[S10]}$$

The scaling (S10) comes from the incompressibility condition, which implies that the pressure is obtained by solving the equation:

$$\nabla^2 p = -\rho\nabla\cdot(\mathbf{v}\cdot\nabla\mathbf{v}). \quad \text{[S11]}$$

Therefore, the scaling (S10) is consistent with the scaling (S8).

The key point is that the scaling (S7)-(S10) describe a turbulent flow with the same Reynolds number Re=$v_{\rm rms}L/\nu$, where $v_{\rm rms}$ is the root-mean-square velocity fluctuation. This is easily obtained using scaling (S8) and (S9). Also the Kolmogorov scale $\eta = [\nu^3/\epsilon]^{1/4}$ (1) is left invariant:

$$\eta = \left[\frac{\nu^3}{\epsilon}\right]^{1/4} = \left[\frac{\lambda^3\tilde{\nu}^3}{v_{\rm rms}^3/L}\right]^{1/4} = \left[\frac{\tilde{\nu}^3}{\tilde{v}_{\rm rms}^3/L}\right]^{1/4} = L\mathrm{Re}^{-3/4}, \quad \text{[S12]}$$

where we use the standard relation for the dissipation rate $\epsilon = v_{\rm rms}^3/L$ (1). In other words, the scaling transformations (S7)-(S10) describe the same turbulent flow with the same dynamics in space but at different times $\tilde{t} = \lambda t$, (i.e., scaling (S7)). By increasing $\lambda$, we speed up the time dynamics of $f$ in Eq. (S1) with respect to the biological time scale $1/\mu$, but the relevant spatial scales, i.e., the Fisher scale $w$ and the inertial range $L/\eta$, are all kept constant.

In summary, by keeping $\mu$ fixed and using Eq. (S1) and Eq. (S2), we are looking at the antagonist dynamics with an equivalent genetic time scale $(\lambda/\mu)$ provided that the spatial scales are kept constant. Thus, for large $\lambda$, the genetic dynamics occurs on a longer time scale with respect to the turbulent flow, whereas for small $\lambda$, the genetic dynamics occur on a faster time scale. It follows that the Damköhler number Da $= \mu L/v_{\rm rms}$ is the meaningful dimensionless number to be considered.

## 2. Measuring the critical fraction for fixation $f_c$

Fig. S1 shows the probability of fixation versus the initialized fraction $f_0$ for different settings of the selective advantage $\delta$ while keeping $\sigma = 0.25$ and Da=1. Every data point is the sample mean over $N = 50$ runs with different turbulent flow fields but an identical Reynolds number and the corresponding standard error. For each setting of $\delta$, we fit a sigmoidal function $P(f) = 1/(1 + \exp[-(f - f_c)/\sigma_p])$ for the fixation probability of the advantageous strain A (dashed lines). On average, strain A, therefore, goes into fixation at least 50% of the cases when $f > f_c$, while $\sigma_p$ quantifies the width of the transition. Note that the obtained values of $f_c$ and $\sigma_p$ depend only weakly on the chosen circular initial condition, as long as the individual initialized objects are larger than $w$, see next section.

## 3. Influence of different initial conditions

In the main text, we always initialized circular patches of strain $A$ in a system filled with strain $B$. Here, we show examples of different initial shapes of these patches and check their consequences on the critical fraction for fixation in Fig. S2(a). We measured the critical fraction $f_0$ for the antagonistic strength $\sigma = 0.25$ and Da=1 as a function of the selective advantage $\delta$ for six different initial conditions, displayed in Fig. S2(b). All initial conditions show a similar quantitative trend and lie within the relative width of their transitions, with the exception of the initial condition of four circles, where each circle is now smaller and closer to the nucleation threshold. The excess perimeter in the latter case thus requires a slightly higher initial fraction for the blue strain to reach fixation. We conclude that the actual shape of the initial shapes just slightly affects the critical fraction of fixation as long as the patches are organized in larger clusters. Nevertheless, the effective theory developed in the main text may still be applicable to the cases of many small initial clusters when mixing time is lowered.

## 4. Temporal evolution of total concentration fluctuations $\langle \delta c_T^2 \rangle$

When passive scalars get turbulently mixed, a cascade of $\langle \delta c_T^2 \rangle$ occurs from large to small scales within the Kolmogorov theory and fluctuations decay like $\langle \delta c_T^2 \rangle \propto \exp(-t)$. Here, we study the fluctuations of the total concentration in antagonistic genetic mixtures.

The equation of motions we consider are:

$$\partial_t c_T + \mathbf{v} \cdot \nabla c_T = D\nabla^2 c_T + \mu c_T(1 - c_T) - 2\mu\sigma c_T^2 f(1 - f) \quad \text{[S13]}$$

where $\mathbf{v}$ is a turbulent field. We introduce the space average $\langle ... \rangle$, and we are interested in understanding the behavior of $\langle c_T^2 \rangle$. For this, we define $\delta c_T = c_T - \langle c_T \rangle$. Upon averaging in space, Eq. (S13) becomes:

$$\partial_t \langle c_T \rangle = \mu \langle c_T \rangle - \mu(\langle c_T \rangle^2 + \langle \delta c_T^2 \rangle) - 2\mu\sigma \langle c_T^2 \rangle H, \quad \text{[S14]}$$

where $H \equiv \langle f(1 - f) \rangle$ is the spatially averaged heterozygosity (2). Here we have assumed that correlations can be factored, so that

$$\langle c_T^2 f(1 - f) \rangle = \langle c_T^2 \rangle \langle f(1 - f) \rangle. \quad \text{[S15]}$$

This is a strong approximation which cannot be true because the spatial variations of $c_T$ are correlated with the regions where $f(1-f)$ is different from 0. Thus, Eq. (S15) should be considered as a valid approximation up to some overall constant, which, for simplicity, we put equal to 1. Nevertheless, Eq. (S15) helps us in understanding the qualitative behavior of $\langle \delta c_T^2 \rangle$.

Using Eq. (S14) and Eq. (S15) we find:

$$\partial_t \langle c_T \rangle = \mu \left[ \langle c_T \rangle - (\langle c_T \rangle^2 + \langle \delta c_T^2 \rangle)(1 + 2\sigma H) \right] \quad \text{[S16]}$$

The equation above tells us that on the time scale of $\mathcal{O}(1/\mu)$, the space average $\langle c_T \rangle$ reaches a stationary value. This is true if we assume that the time behavior of $H$ is slower than the time needed for $\langle c_T \rangle$ to reach the (almost) stationary value. In the following, we also assume that $\langle \delta c_T^2 \rangle$ is a relatively small quantity, and we can neglect terms of order $\mathcal{O}(\delta c_T^3)$. With this, the first order in $\langle \delta c_T^2 \rangle$ reads:

$$\langle c_T \rangle = \frac{1}{1 + 2\sigma H} - (1 + 2\sigma H) \langle \delta c_T^2 \rangle. \quad \text{[S17]}$$

Using Eq. (S13) and Eq. (S16), we can now write the equation for $\delta c$ as

$$\partial_t \delta c_T = D\nabla^2 \delta c_T + \mu \delta c_T (1 - \langle c_T \rangle) - \mu \langle \delta c_T^2 \rangle - 2\mu\sigma(2\langle c_T \rangle - \langle \delta c_T^2 \rangle) H + \mathcal{O}(\delta c_T^2) \quad \text{[S18]}$$

Multiplying Eq. (S18) by $\delta c_T$, using Eq. (S17) and performing the space average, we finally obtain

$$\frac{1}{2} \partial_t \langle \delta c_T^2 \rangle = -D \langle (\nabla \delta c_T)^2 \rangle - \frac{2\mu\sigma H}{1 + 2\sigma H} \langle \delta c_T^2 \rangle \quad \text{[S19]}$$

which is our final result. Because of the different assumptions, Eq. (S15), and approximations, we should consider Eq. (S19) as a tool to understand the qualitative behavior of $\langle \delta c_T^2 \rangle$ in time. The key observation is that we expect $\delta c_T$ to be significantly large locally in space in the regions where $f(1-f)$ is large, i.e., at the interface of the two populations. Then, it is reasonable to argue that the first term on the RHS of Eq. (S19) is proportional to $H/l^2$ where $l$ is the size of the interface (i.e., $w$ for a sharp interface). Thus, up to some constant, we reach the conclusion that $\langle \delta c_T^2 \rangle$ should decay in time at a rate proportional to $H$.

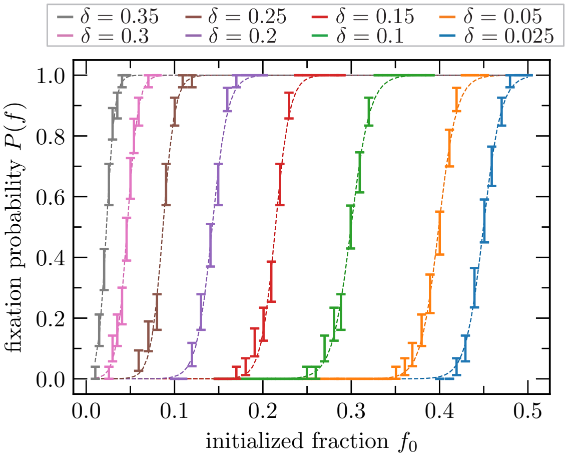


**Fig. S1.** Measured fixation probability for different selective advantages $\delta$ with error bars coming from the standard error from $N = 50$ runs of different fluid flows with Da=1. Furthermore, we show the fitted sigmoidal functions as dashed lines.

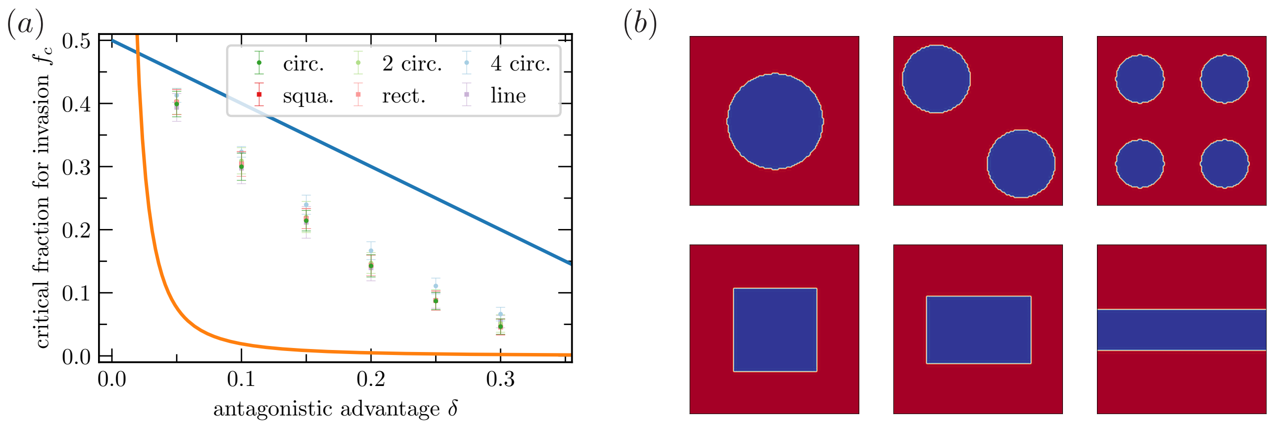


**Fig. S2.** Study of the influence of initial conditions on the critical fraction of fixation. Similar to Fig. 2 (b), we numerically measured $f_c$ for (a), for six different initial conditions shown in (b). Furthermore, we show $f_c^0$ (blue line) and $f_c^\infty$ (orange line).

| Parameter table | | | | | | | | |
|---|---|---|---|---|---|---|---|---|
| | $L$ | $\eta$ | $\mu$ | $D$ | Da | $\sigma$ | $\delta$ | $f_0$ |
| Fig. 1(a) | $2\pi$ | $0.0024$ | n.a.[†] | $0.0024$ | a.i.[*] | n.a.[†] | n.a.[†] | 0.2 |
| Fig. 1(b) | $2\pi$ | $0.0024$ | $1.0$ | $0.0024$ | a.i.[*] | 0.25 | 0.1 | 0.2 |
| Fig. 1(c) | $2\pi$ | $0.0024$ | n.a.[†] | $0.0024$ | a.i.[*] | n.a.[†] | n.a.[†] | 0.2 |
| Fig. 2(a) | $2\pi$ | $0.0024$ | $1.0$ | $0.0024$ | a.i.[*] | 0.25 | 0.1 | a.i.[*] |
| Fig. 2(b) | $2\pi$ | $0.0024$ | $1.0$ | $0.0024$ | a.i.[*] | 0.25 | a.i.[*] | n.a.[†] |
| Fig. 3(a) | $2\pi$ | $0.0024$ | $1.0$ | $0.0024$ | a.i.[*] | 0.25 | 0.1 | a.i.[*] |
| Fig. 3(b) | $2\pi$ | $0.0024$ | $1.0$ | $0.0024$ | 0.1 | 0.25 | 0.1 | 0.05 |
| Fig. 3(b) inset | $2\pi$ | $0.0024$ | $1.0$ | $0.0024$ | 1.0 | 0.25 | 0.1 | 0.3 |
| Fig. 3(c) | $2\pi$ | $0.0024$ | $1.0$ | $0.0024$ | 0.1 | 0.25 | 0.1 | 0.05 |
| Fig. 3(d) | $2\pi$ | $0.0024$ | $1.0$ | $0.0024$ | n.a.[†] | a.i.[*] | n.a.[†] | n.a.[†] |
| Fig. 4(a) | $2\pi$ | $0.0024$ | n.a.[†] | n.a.[†] | n.a.[†] | n.a.[†] | n.a.[†] | n.a.[†] |
| Fig. 4(b) | $2\pi$ | $0.0024$ | $1.0$ | $0.0024$ | 0.1 | 0.25 | 0.1 | 0.2 |
| Fig. 4(c) | $2\pi$ | $0.0024$ | $1.0$ | $0.0024$ | 0.1 | 0.25 | 0.1 | 0.2 |
| Fig. 4(d) | $2\pi$ | $0.0024$ | $1.0$ | $0.0024$ | 10.0 | 0.25 | 0.1 | 0.2 |
| Fig. S1 | $2\pi$ | $0.0024$ | $1.0$ | $0.0024$ | 1.0 | 0.25 | a.i.[*] | a.i.[*] |
| Fig. S2(a) | $2\pi$ | $0.0024$ | $1.0$ | $0.0024$ | 1.0 | 0.25 | a.i.[*] | n.a.[†] |
| Fig. S2(b) | $2\pi$ | n.a.[†] | n.a.[†] | n.a.[†] | n.a.[†] | n.a.[†] | n.a.[†] | 0.25 |

[*] as indicated in the corresponding figure/figure caption

[†] not applicable

**Table S1.** All simulations were done by solving the Navier-Stokes equation first via spectral methods and random forcing at long scales. The generated velocity fields were used as inputs for a finite difference scheme on a two-dimensional square lattice with 128 lattice sites in each direction. We scaled the velocity field such that the corresponding Damköhler number was achieved.

**Movie S1.** Movies of the concentration field of a passive scalar on the left, the field of fraction $f$ for different Damköhler numbers in the middle, and the concentration field of a binary phase separating mixture on the right under turbulent mixing. All systems are stirred with the same turbulent flow field and shown in units of the large eddy turnover time. Additionally, we show the critical nucleation radius (white circle) in the genetic mixtures in the absence of flow. In all systems, we use a circular initialization that covers 20% of the system size (blue circle/first column). In Fig. 1, we show selected time points of this dynamics.

## References


1. U Frisch, *Turbulence: the legacy of AN Kolmogorov.* (Cambridge university press), (1995).
2. KS Korolev, M Avlund, O Hallatschek, DR Nelson, Genetic demixing and evolution in linear stepping stone models. *Rev. modern physics* **82**, 1691–1718 (2010).
